# Supplementary material for: Reconfigurable Intelligent Surface-Based Index Modulation: A New Beyond MIMO Paradigm for 6G
Source: arXiv:1904.06704 source file (2020-01-29)
Supplement: Supplementary file 1 [file LIS_SSK_SM.pdf]

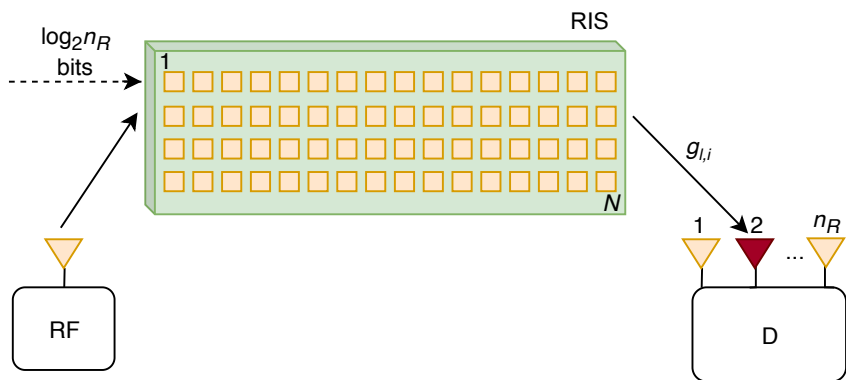

(a)

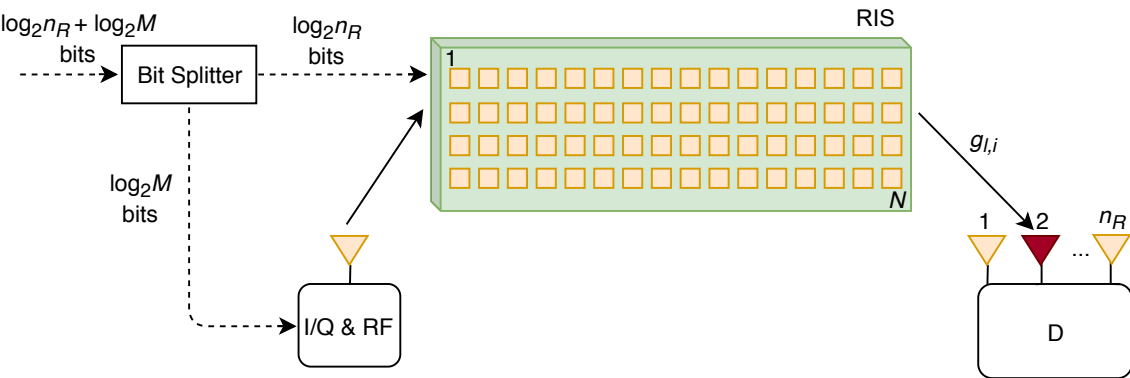

(b)
